# Supplementary material for: Uniform Object Rearrangement: From Complete Monotone Primitives to Efficient Non-Monotone Informed Search
Source: arXiv:2101.12241 source file (2022-03-18)
Supplement: Supplementary file 1 [file 10_appendix.tex]

\section{Appendix}
\label{sec:appendix}

\begin{proposition}
\label{prop:space-rg}
Let $\mathbf{C}$ be the set of continuous curves $[0,1] \mapsto \workspace$ and $G_\arrangement = (\mathcal{R_\arrangement}, E)$ a region graph given arrangement $\arrangement$ for object $o_i$. Then $\exists! \mathcal{S}: \mathbf{C} \to W_{G_\arrangement}$, where $W_{G_\arrangement}$ is the set of all walks on $G_\arrangement$. 
\end{proposition}

\begin{proof}
The proof is by construction. Let $T:\workspace \to \mathcal{R_\arrangement}$ map points on the interior of a region $r \in \mathcal{R_\arrangement}$ to that corresponding region. $\mathcal{S}$ maps continuous segments of a curve $\pi \subset \workspace$ that lie in the interior of a region to the empty sequence.

Fix $p \in \pi$ to be a point on the boundary of 2 or more regions and let $i \in [0,1]$ such that $\pi(i)=p$. For any $\epsilon > 0$, let the segment $\pi_\epsilon$ be the restriction of $\pi$ on the interval $(i-\epsilon,i+\epsilon)$. Without loss of generality, $\mathcal{S}$ maps the segment $\pi_\epsilon$ to the singleton edge sequence containing $$e = \left(\lim_{x\to i^-}T(x),\lim_{x\to i^+}T(x)\right)$$
The map $\mathcal{S}$ is now well defined for any continuous curve by decomposing the curve into a sequence of segments internal to a region and crossing region boundaries and then applying the definitions segment-wise.
See figure~\ref{fig:segments} for a basic example.
\end{proof}

\begin{figure}[ht]
    \centering
    \includegraphics[width=\linewidth]{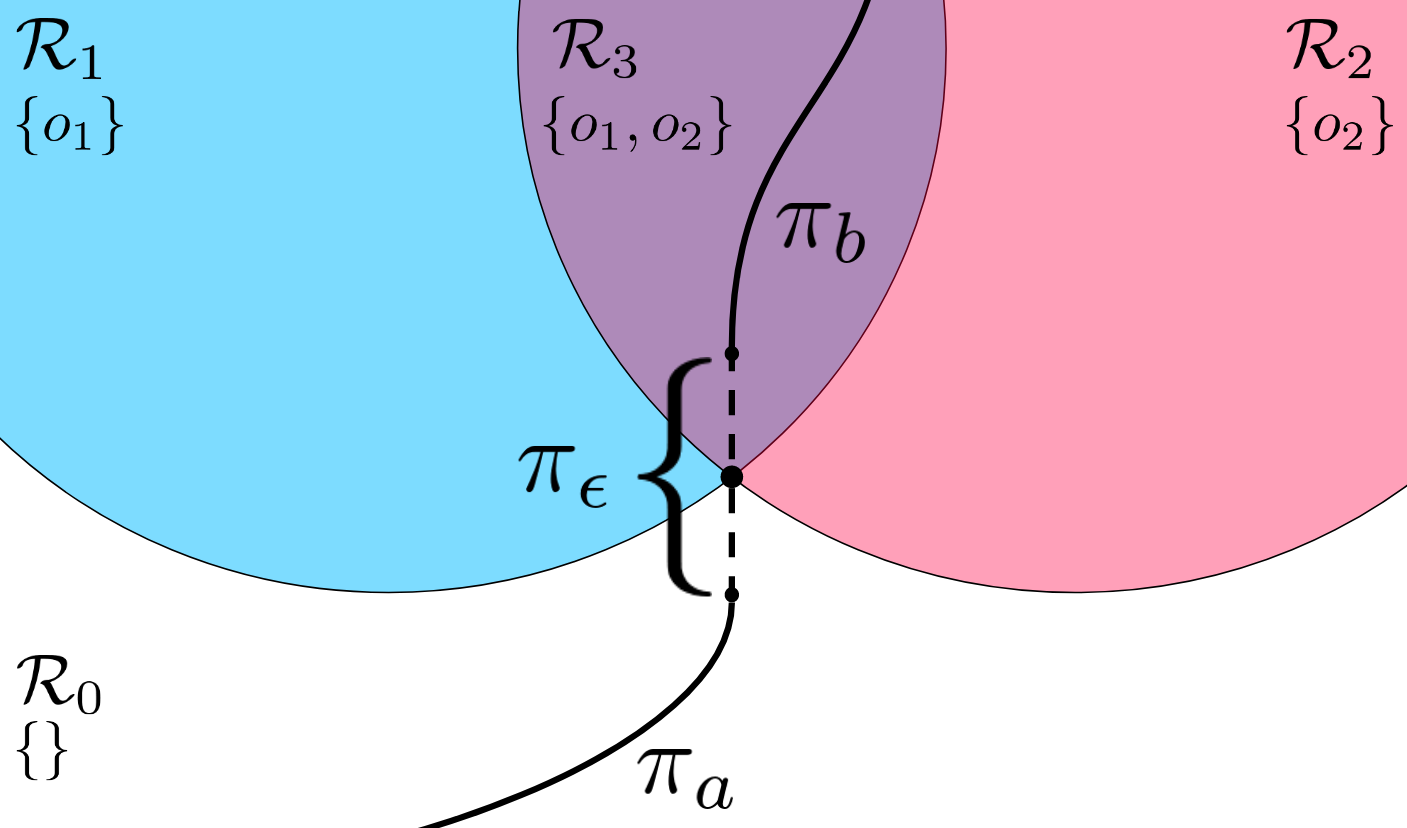}
    \caption{A curve is decomposed into segments $\pi_a$, $\pi_\epsilon$, and $\pi_b$. $\mathcal{S}$ maps each segment to $\emptyset$, $(e = (\mathcal{R}_0,\mathcal{R}_3))$, and $\emptyset$ respectively. The interference set for the shown curve is $\mathbf{I}(\pi_\epsilon)=\mathbf{I}(\mathcal{R}_0) \cup \mathbf{I}(\mathcal{R}_3) =\{o_1, o_2\}$}
    \label{fig:segments}
\end{figure}

\begin{corollary}
\label{cor:interference_rg}
$\mathbf{I}(\pi) = \mathbf{I}(\mathcal{S}(\pi))$
\end{corollary}

\begin{proof}
Recall the construction of the map of $\mathcal{S}$. Any segment of a curve on the interior of a region has the same interference set as that region by definition. Every edge $e \in \mathcal{S}(\pi)$ is defined from segments interior to 2 regions straddling a shared boundary point. Since all regions are accounted for taking the union of their interference sets accounts for all the points of $\pi$.
% Make better using the T function.
\end{proof}

\begin{corollary}
\label{cor:psuedo-inverse_rg}
There exists many $\mathcal{Q}: W_{G_\arrangement} \to \mathbf{C}$
\end{corollary}

\begin{proof}
First note that since region in $\mathcal{R_\arrangement}$ are path connected by definition. Thus for any vertex in a walk on $G_\arrangement$ a continuous curve exists in the corresponding region connecting some point on the shared boundary of the previous vertex to a point on the shared boundary of the next vertex. By concatenating one of each such curves for all vertices along the walk you can construct a continuous curve to correspond to the entire walk.
\end{proof}

%\begin{proposition}
%A BFS on $G_\arrangement$ from root $r \in \mathcal{R}_\arrangement$ accounts for all simple curves starting at points in $r$ and ending in points of every other region.
%\end{proposition}

\begin{figure}
    \centering
    \includegraphics[width=0.99\linewidth]{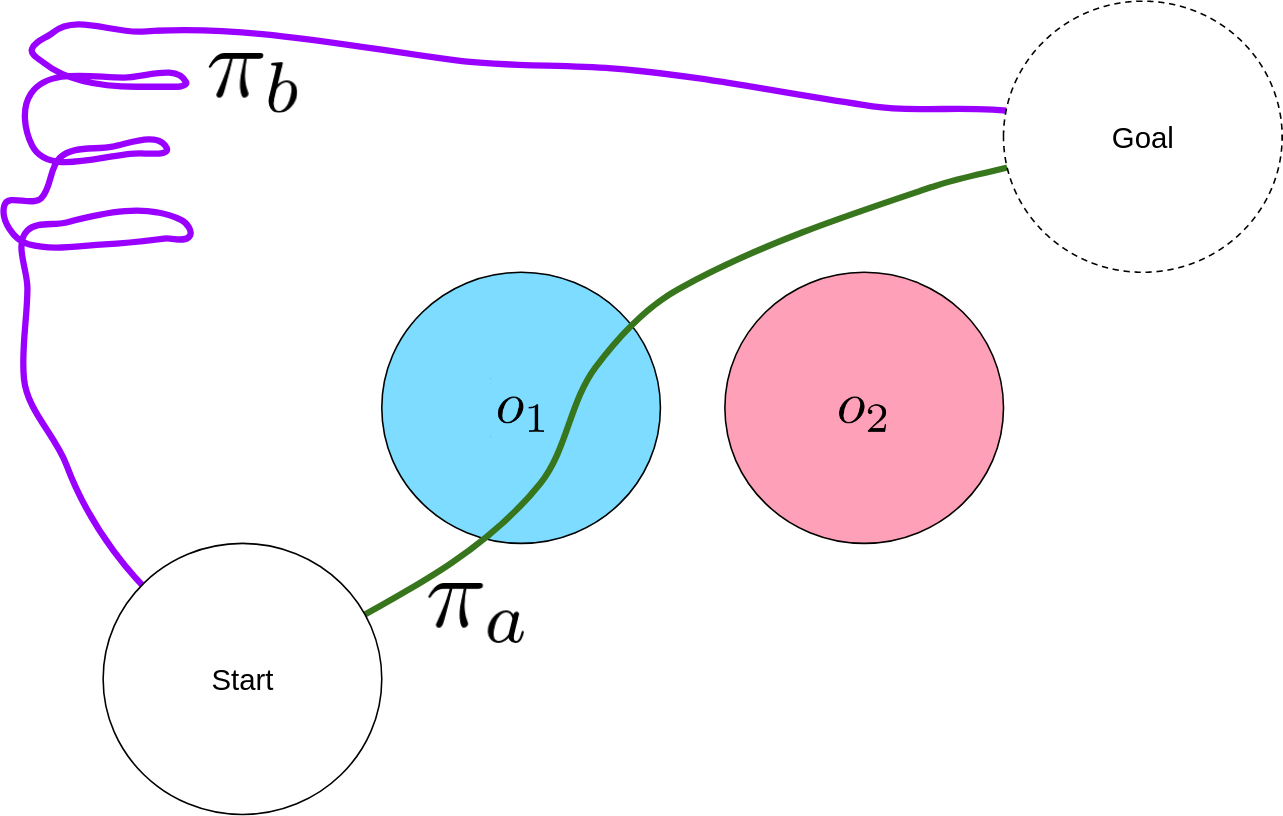}
    $$\empty$$
    \includegraphics[width=0.99\linewidth]{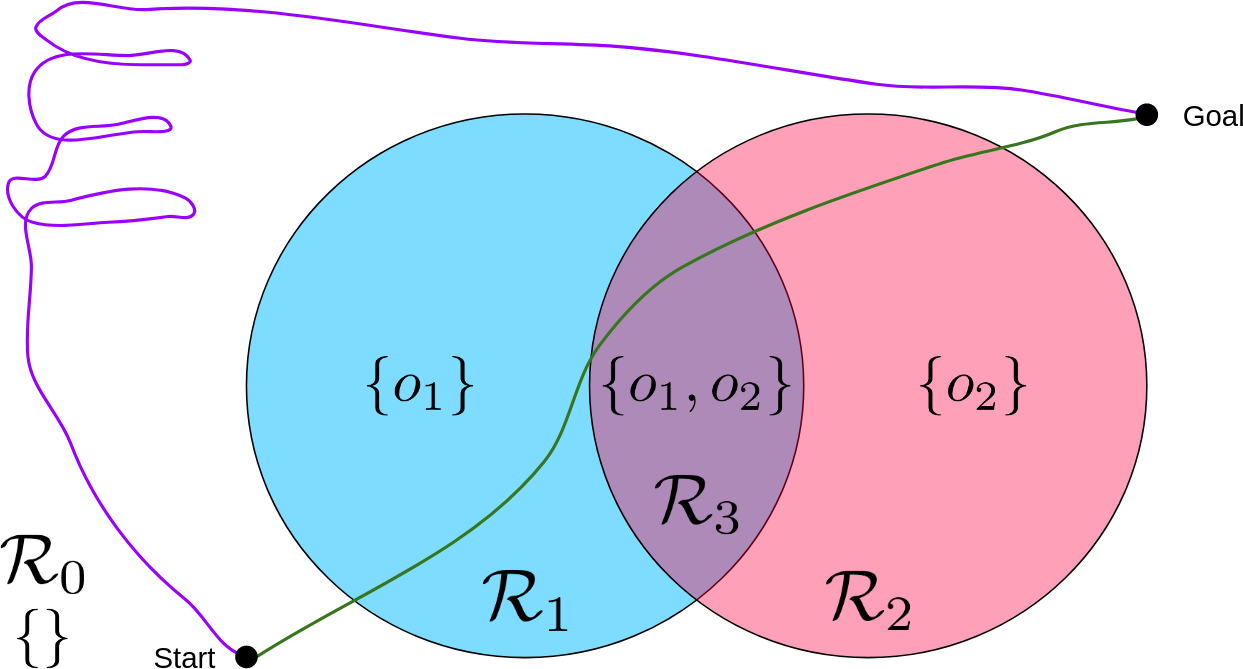}
    $$\empty$$
    \includegraphics[width=0.99\linewidth]{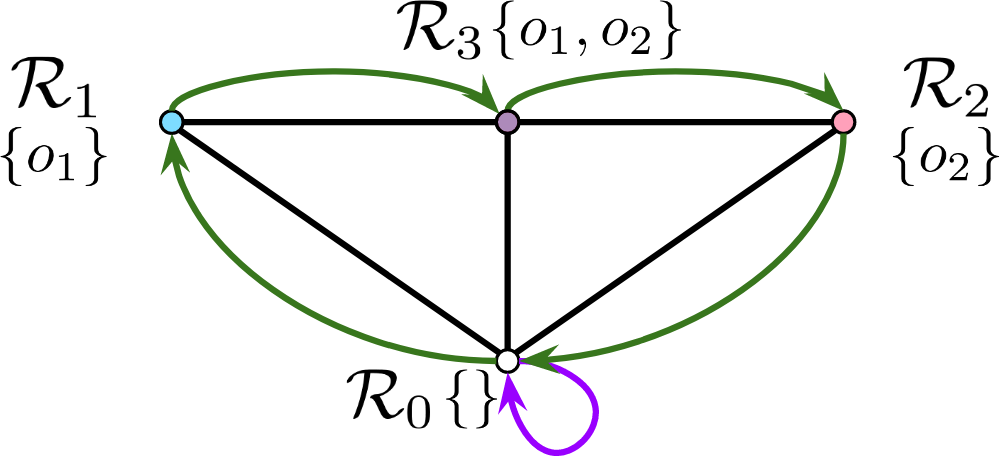}
    \caption{A workspace with three disks is shown on top. With a start and goal specified for one of the disks. Two paths are drawn, a green colliding path and a purple free path. In the middle the configuration space for the selected object is shown decomposed into regions of unique interference. On the bottom is the resulting region graph with colored arcs tracing along path in the region graph corresponding to the paths of the respective color in the workspace.}
    \label{fig:workspace2regions}
\end{figure}

\textbf{(1) Object Rearrangement Problems} Object rearrangement problems can be categorized based on object-object and object-arm interaction during the execution. One class of such problems is tabletop arrangement, where objects are approached and transferred in a tabletop manner. Since it assumes no object-arm interactivity, more emphasis is laid on minimizing the travel distance of the end-effector, instead of collision avoidance. 
The problem is modelled as a travelling salesman problem (TSP) \cite{han2018complexity} in the case where start and goal poses of objects do not overlap. Object-object interaction is considered in the overlapping cases, where a reduction from feedback vertex set is performed to minimize the total pick-and-place actions \cite{han2018complexity}. The problem considered here has a harder condition of object-object interaction, where a transferring path of a certain object may overlap with other objects' poses. Dual arm systems potentially facilitate rearrangement tasks but introduce more complexity. The idea is to first figure out the best pair assignment of the objects using optimal matching and then determine the ordering of pairs \cite{shome2018fast}. Again, it assumes monotonicity and object non-interactivity which can not be waived in the harder setup considered here. There are also a few works on tabletop object placement and rearrangement that, like this work, seek to minimize the number of actions taken \cite{havur2014geometric, dabbour2019placement}. They use answer set programming (ASP) to find an optimal discretization which they use to find a sequence of actions to satisfy a final arrangement.

A more general rearrangement than tabletop rearrangement performs in a confined environment (e.g., shelf, box) where overhand grasp is disabled. In this case, object-object and object-arm interaction cannot be waived due to geometric constraints. The ordering of transferring objects is crucial to avoid collision.
One approach is to search over all possible orders with which the objects are transferred \cite{stilman2007manipulation}. This approach only works for monotone instances and is not scalable when the number of objects increases. A dependency graph \cite{van2009centralized} can be introduced to describe the constraints occurring between different objects, upon which the execution sequence of moving objects can be determined. Minimum constraint removal (MCR) paths \cite{hauser2014minimum}\cite{hauser2013minimum}, which give an explanation as to what constraints are violated along the paths, are often used as heuristics for constructing dependency graphs \cite{krontiris2016efficiently}. Non-monotone problems have been approached by integrating efficient monotone solvers into high-level incremental search algorithms such as building a PRM or Bi-RRT \cite{krontiris2016efficiently}\cite{krontiris2015dealing}. These works suffer from the random nature of the sampling-based methods, which can be improved by applying heuristics to guide the sampling process. In addition, scalability of the approaches remains further discussion. Object rearrangement can also be treated as task and motion planning, where symbolic planners can be used to construct a plan \cite{garrett2015ffrob}\cite{srivastava2014combined}. 

Object arrangements can also be fulfilled by non-prehensile operations on the objects such as pushing actions. The pushing planning enables simultaneous manipulation of several objects \cite{ben1995push}\cite{ben1998practical} and handles heavy objects which cannot be easily lifted. On the other hand, the pushing actions are irreversible and unpredictable, which often results in low-quality arrangement along the way. \cite{huang2019large} proposes a tabletop rearrangement system which handles large-scale multi-object rearrangements by pushing actions. Pushing actions are increasingly used in object rearrangement under uncertainty, e.g., planning a
sequence of primitive actions (e.g. pushing) to manipulate the objects
to the desirable arrangement \cite{dogar2012planning},
\cite{koval2015robust}.  The problem is treated as belief-state
planning and such belief-state transition models can be learned prior
to planning \cite{anders2018reliably} to tackle pushing multi-object
rearrangement.

\textbf{(3) NAMO and Retrieval Problem}
NAMO (Navigation Among Movable Obstacles) and the retrieval problem are two related challenges to rearrangement planning. Both of them need to relocate movable obstacles before the manipulator or the mobile robot reaches its target. 
NAMO was first addressed by Chen and Hwang \cite{chen1990practical}. Stilman and Kuffner \cite{stilman2008planning} proved the NP-hardness of the problem and categorized NAMO problems based on linearity and monotonicity. In the $L_k$ problems, at most $k$ objects need to be displaced to merge two components. And in the monotone problems, each object can be moved at most once. Besides that, a resolution complete algorithm is given for problems in the class $L_kM$. For the non-monotone non-linear NAMO problems, Van den Berg et al. \cite{van2009path} proposed a probabilistically complete algorithm assuming that all the objects and the robot are axis-aligned rectangles. However, the algorithm is inefficient with lots of unnecessary object movements. Recently, there have also been some papers \cite{wu2010navigation}, \cite{kakiuchi2010working}, \cite{levihn2014locally} published on online NAMO, where the robot dynamically modifies the plan in an unknown environment. In object retrieval problems, in order to retrieve a target object, obstacles obstructing the path towards the target have to be relocated \cite{dogar2012planning}. Recently, algorithms \cite{nam2019planning}\cite{nam2020fast} have been proposed to minimize the number of objects to relocate.

\textbf{(4) Buffer selection}
For non-monotone problems where certain object has to be put temporarily in an intermediate configuration (called a buffer) before moving to the goal configuration, it is very important to determine where to put certain objects which can minimize further actions. A systematic way to determine the best buffer has been introduced \cite{cheong2020relocate} based on the number of valid slots that could be occluded if a certain object is placed in this buffer. (can add more references when I reach there)

\textbf{(4) Multi-robot multi-object rearrangement} Multi-robot multi-object rearrangement problems have also been studied. In the domain of mobile robots, rearrangement problems are often referred to as pickup and delivery (PDP) problems \cite{parragh2008survey}. In such a setup, task constraints (i.e. the order of starting and finishing time) must be taken into account to decide the order of task execution. These task constraints are selectively calculated step by step \cite{fujii2008rearrangement} so as to save high computational cost. Combinatorial challenges are examined and tamed in clutter removal tasks using mobile robots with manipulators \cite{tang2019taming}. The search space in multi-robot multi-object rearrangement is usually large and can be reduced \cite{levihn2012multi} by splitting the planning into different stages including robot traversal and object assignments to robots.  

\textbf{(4.5) Computational Geometry}
Varieties of labeled and unlabeled disc rearrangement problems have been studied in \cite{bereg2008sliding} and efficient algorithms motivated for multi-robot systems have been proposed in \cite{solomonmotion,adler2015efficient}. These works study a different variation of the problem than we are interested in however. While these previous works are focused on low complexity algorithms where multiple robots can move at the same time, we are motivated by an environment where a robot can only manipulate one object at a time. Thus we will consider a restricted disc rearrangement problem where only one disc can move at a time. Furthermore, rather than minimizing path length we wish to minimize the number of actions.
In this work, we propose a graph construction of regions that is very similar to one proposed for coordinating the motion of independent circular bodies \cite{schwartz1983piano}. The complexity of constructing the connectivity graph proposed in that work scales rapidly with the number of objects considered (practically infeasible $>3$). Due to the restriction of only moving one object at a time, we are able to combat scaling issues by constructing multiple lower dimensional ``region graphs'' for each individual mobile object rather than one composite connectivity graph for the whole problem instance.

\textbf{(5) Others (temporarily put it here)} A critical challenge in multi-arm motion planning is how to utilize asynchronous and synchronous behaviors of the system to guarantee efficient solutions while minimizing the risk of collisions among the arms and the objects. Some work has been conducted on developing coordination control strategies for a multi-arm system to grab moving objects in a synchronous or asynchronous manner \cite{mirrazavi2018unified}. An extension of the work has been further discussed in the face of uncertainty \cite{sina2016coordinated}. The focus of the work is limited to the coordination of the arms when pick-up takes place. Rearrangement under uncertainty is also modelled as planning a sequence of primitive actions (e.g. pushing) to manipulate the objects to the desirable arrangement \cite{koval2015robust}, \cite{dogar2012planning}.

\textbf{(6) Complete Approaches for Related Problems} In the area of manipulation planning, generalized approaches based on the manipulation graph, where each node on the graph is a configuration of the manipulator and the movable objects, were proposed\cite{alami1994two}\cite{alami1990geometrical}\cite{laumond1989geometrical} to obtain completeness and optimality. However, due to the high computational complexity, the method fails to solve problems with a large number of movable objects. For the grasping problem in a shelf, A. Krontiris et al.\cite{krontiris2015dealing} proposed a probabilistic complete approach based on PRM(Probabilistic Roadmaps)\cite{kavraki1996probabilistic} and RRT(Rapidly-exploring Random Tree)\cite{lavalle1998rapidly}. For the tabletop setup, S. D. Han et al. used dependency graph\cite{van2009centralized} to guarantee completeness and optimality. Besides grasping, numerous works focused on pushing planning problems. O. Ben-Shahar and E. Rivlin presented a resolution complete potential-field method\cite{ben1995push}\cite{ben1998practical} for a object rearrangement problem where a mobile robot inside the workspace moves movable objects by pushing. Completeness is also well-studied in NAMO(Navigation among Movable Obstacles) problems. Resolution complete algorithms were proposed for problems in $L_1$\cite{stilman2005navigation}, where only one object must be displaced to merge two components, and problems in $L_kM$\cite{stilman2008planning}, where at most $k$ objects need to be displaced to merge two components and each object can be moved at most once. And for simple robots(2-3 DOFs), J. van den Berg et al.\cite{van2009path} presented a probabilistic complete method for NAMO problems.
